# Supplementary material for: Accelerating Score-based Generative Models with Preconditioned Diffusion Sampling
Source: arXiv:2207.02196 source file (2022-12-05)
Supplement: Supplementary file 2 [file ffhq_hq.tex]

\begin{figure}[h]
    \vspace{-22ex}
    \centering
    \begin{minipage}{1\linewidth}
        \centerline{\includegraphics[scale=0.26]{pictures_sm/ffhq_ncsnpp_hq.pdf}}%\hspace{3ex}
        \vspace{-10.75ex}%12
    \end{minipage}
    \vspace{-34ex}
        \caption{
        Facial images at a resolution of $1024\times 1024$ generated by NCSN++~\cite{song2020score}
        with our PDS.
        Sampling iterations: $66$.
        Dataset: FFHQ~\cite{karras2019style}.
        }
        \label{fig:ffhq_hq}
\end{figure}
