# Supplementary material for: Accelerating Score-based Generative Models with Preconditioned Diffusion Sampling
Source: arXiv:2207.02196 source file (2022-12-05)
Supplement: Supplementary file 3 [file mnist.tex]

\begin{figure}[ht]
    \vspace{-4ex}
    \centerline{\includegraphics[scale=0.33]{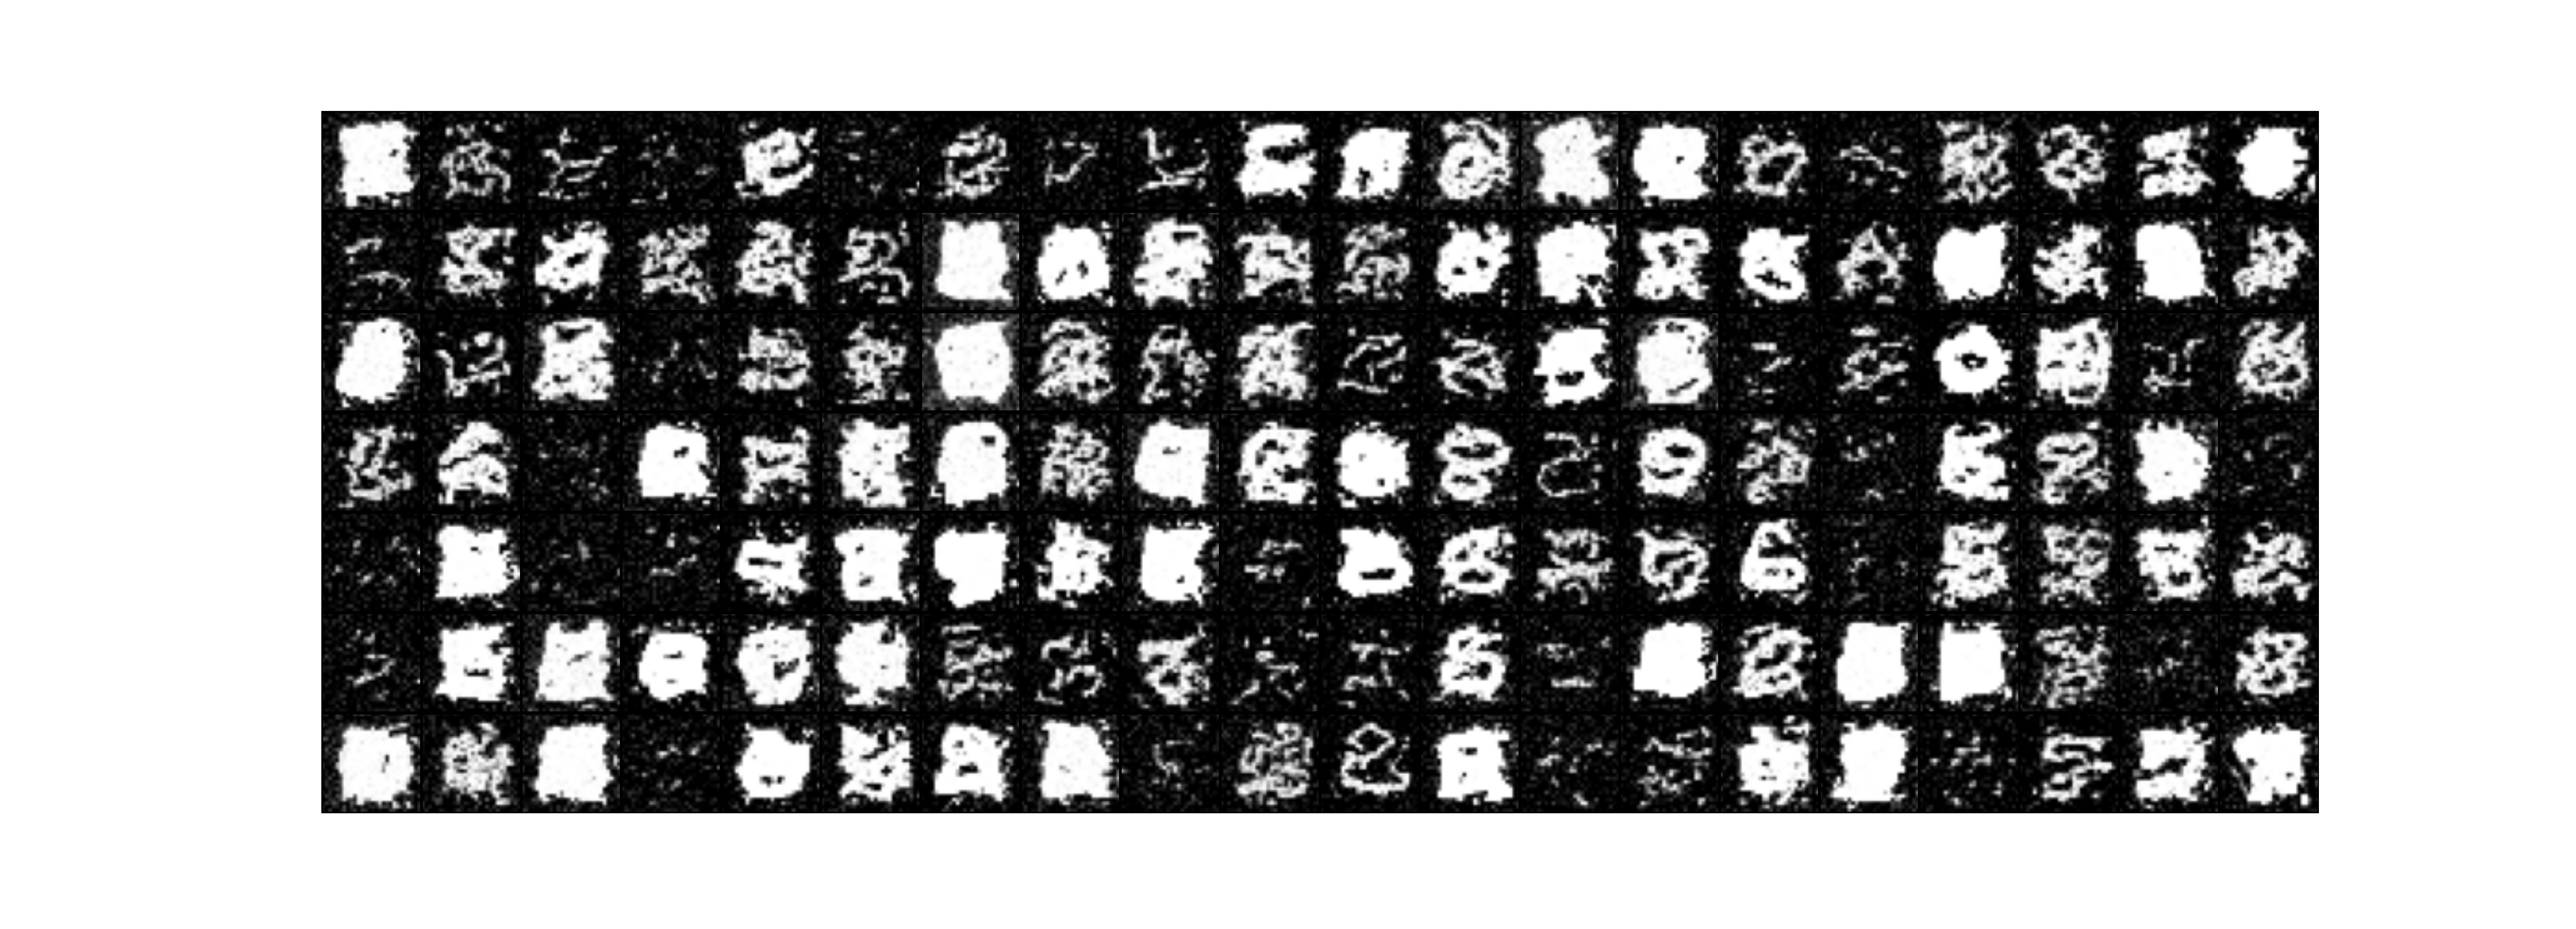}}
         \vspace{-9.8ex}
        \centerline{\includegraphics[scale=0.33]{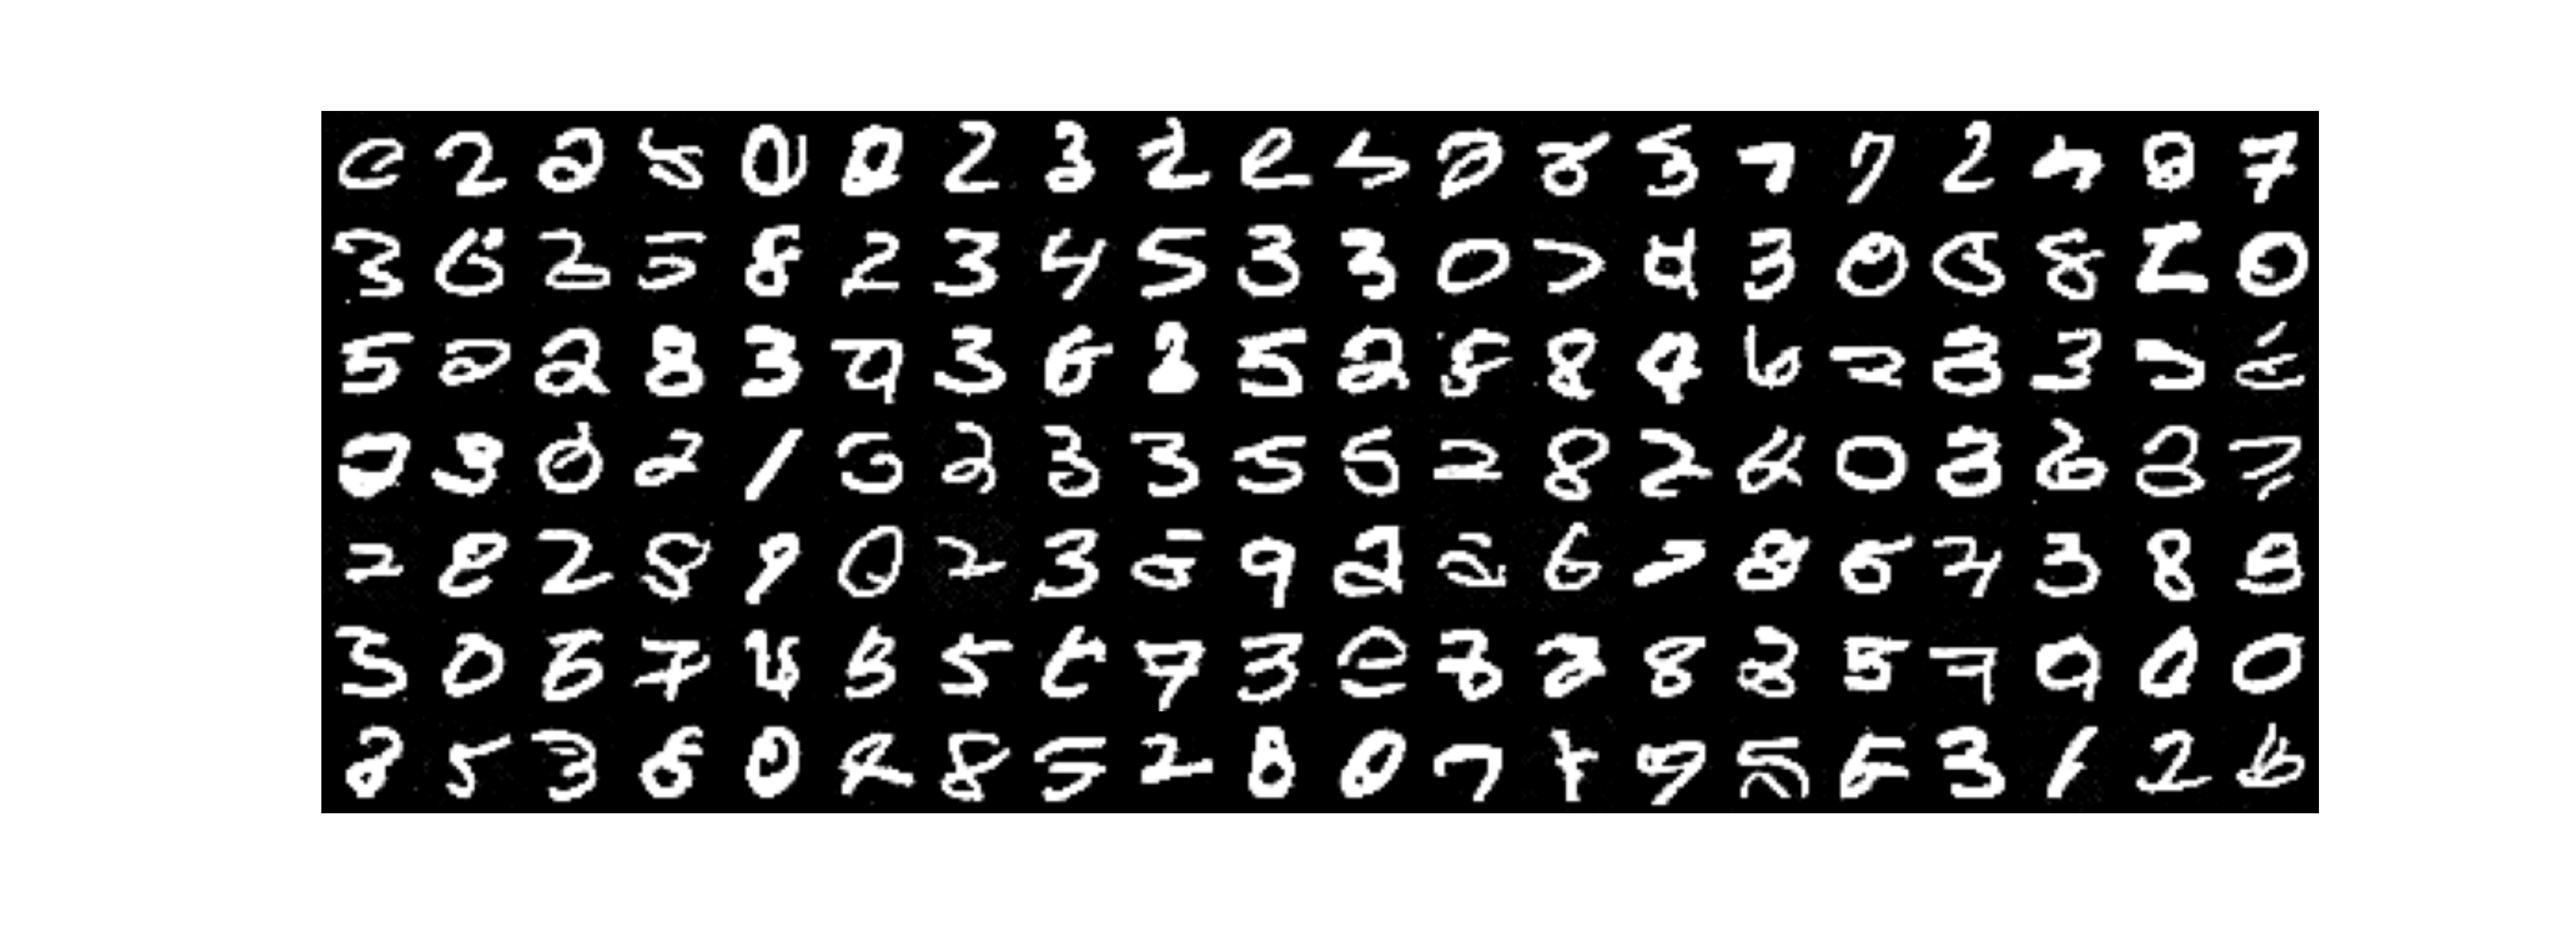}}
    \vspace{-3ex}
        \caption{Sampling using NCSN~\cite{song2019generative} on MNIST ($28 \times 28$). \textbf{Top}: Results by the original sampling method with $20$ sampling iterations. \textbf{Bottom}: Results by our PDS with $20$ sampling iterations, where we set $(r,\lambda)=(0.2H,1.6)$. 
        }      
        \label{fig: mnist_sm}
        \vspace{-6ex}
\end{figure}
