# Supplementary material for: Accelerating Score-based Generative Models with Preconditioned Diffusion Sampling
Source: arXiv:2207.02196 source file (2022-12-05)
Supplement: Supplementary file 5 [file ncsnv2.tex]

\begin{figure}[ht]
    \vspace{-17ex}
    \begin{minipage}{1\linewidth}
        \textcolor{white}{------}\hspace{1ex}$T = 210$\hspace{6ex}$T = 157$\hspace{6ex}$T = 126$\hspace{7ex}$T = 108$\hspace{6ex}$T = 81$\hspace{6ex}$T = 65$
    \vspace{-26ex}
    \end{minipage}
    
    \rotatebox{90}{\textcolor{white}{------}\hspace{-34ex} Ours \hspace{46ex} Baseline~\cite{DBLP:conf/nips/0011E20}} \hspace{-0.5ex}%4
    \begin{minipage}{0.47\linewidth}
        \centerline{\includegraphics[scale=0.24]{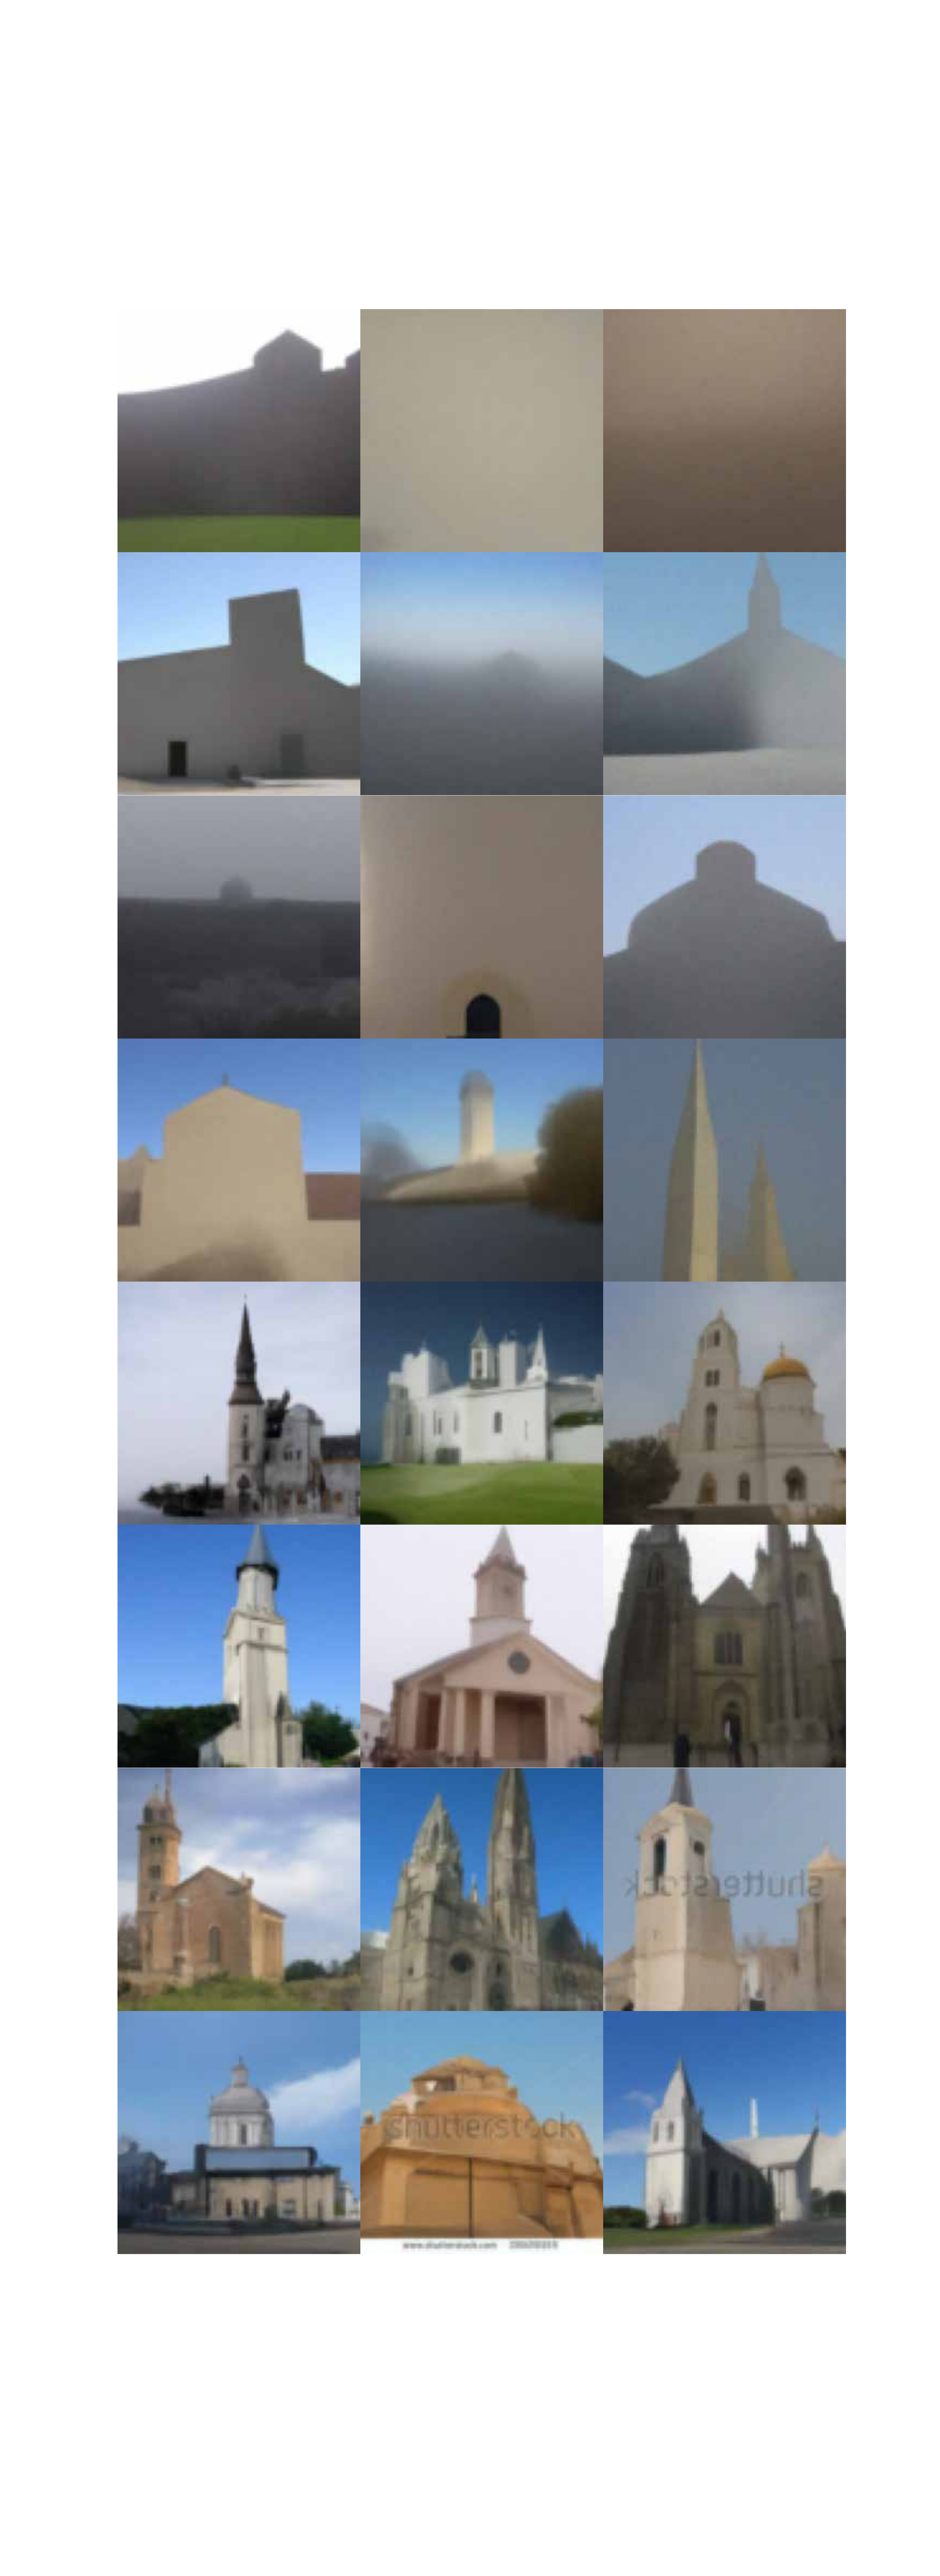}}
    \end{minipage}
    \begin{minipage}{0.47\linewidth}
            \centerline{\includegraphics[scale=0.24]{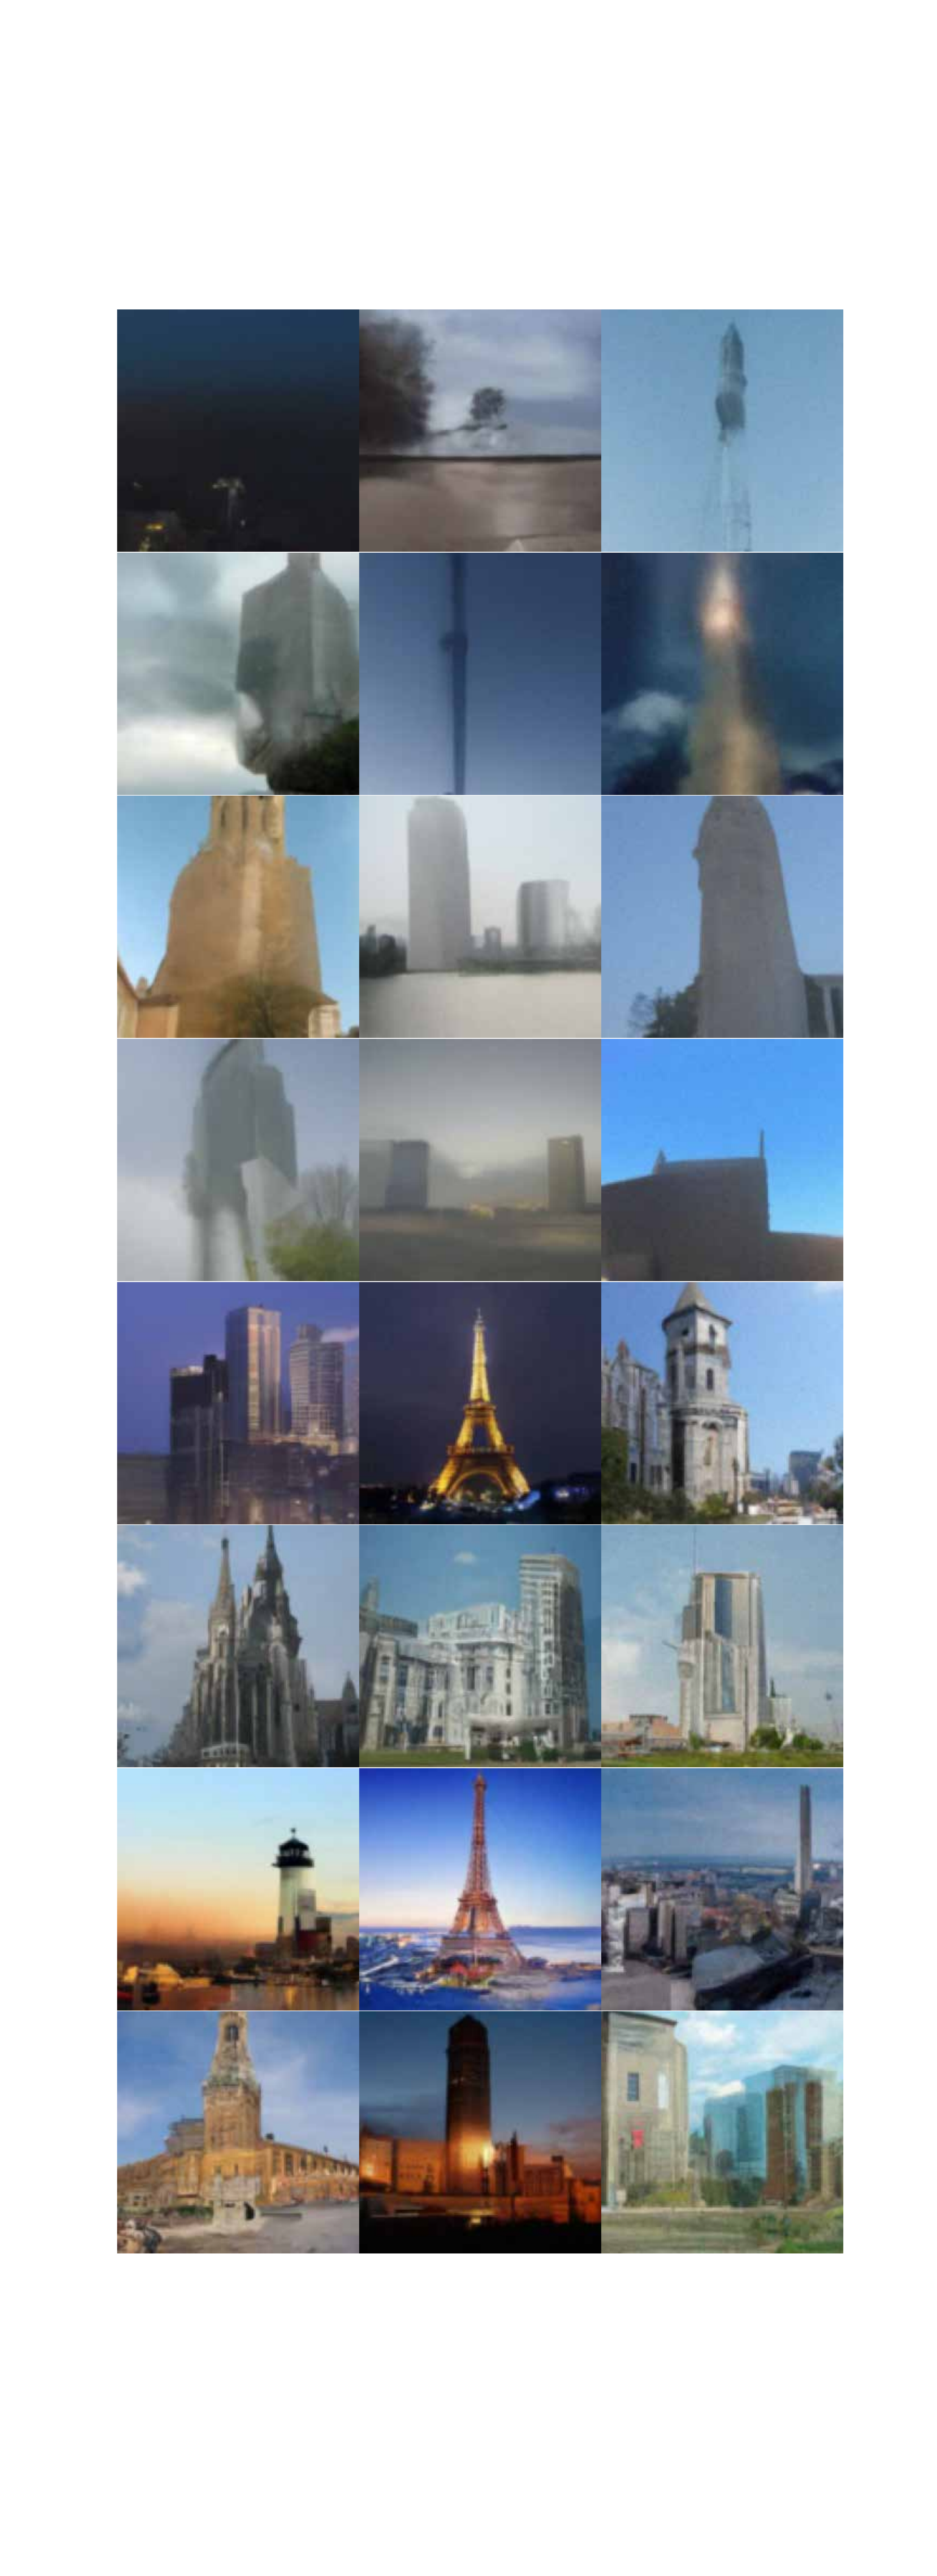}}
    \end{minipage}
    \vspace{-16ex}
           \caption{Sampling using NCSNv2~\cite{DBLP:conf/nips/0011E20} on LSUN (church $96\times 96$ and tower $128 \times 128$) under different iteration numbers.}
        \label{fig: ncsnv2_lsun}
        \vspace{-6ex}
\end{figure}
