# Supplementary material for: Accelerating Score-based Generative Models with Preconditioned Diffusion Sampling
Source: arXiv:2207.02196 source file (2022-12-05)
Supplement: Supplementary file 6 [file solenoidal.tex]

\begin{figure}[H]
    \vspace{-12ex}
    \centering
    \begin{minipage}{1\linewidth}
        \textcolor{white}{------}\hspace{3ex}$S_1$\hspace{12.5ex}$S_2$\hspace{12.5ex}$S_3$\hspace{12.5ex}$S_4$\hspace{12.5ex}$S_5$\hspace{12.5ex}$S_6$
    \vspace{-24ex}
    \end{minipage}
    \begin{minipage}{1\linewidth}
        \centerline{\includegraphics[scale=0.21]{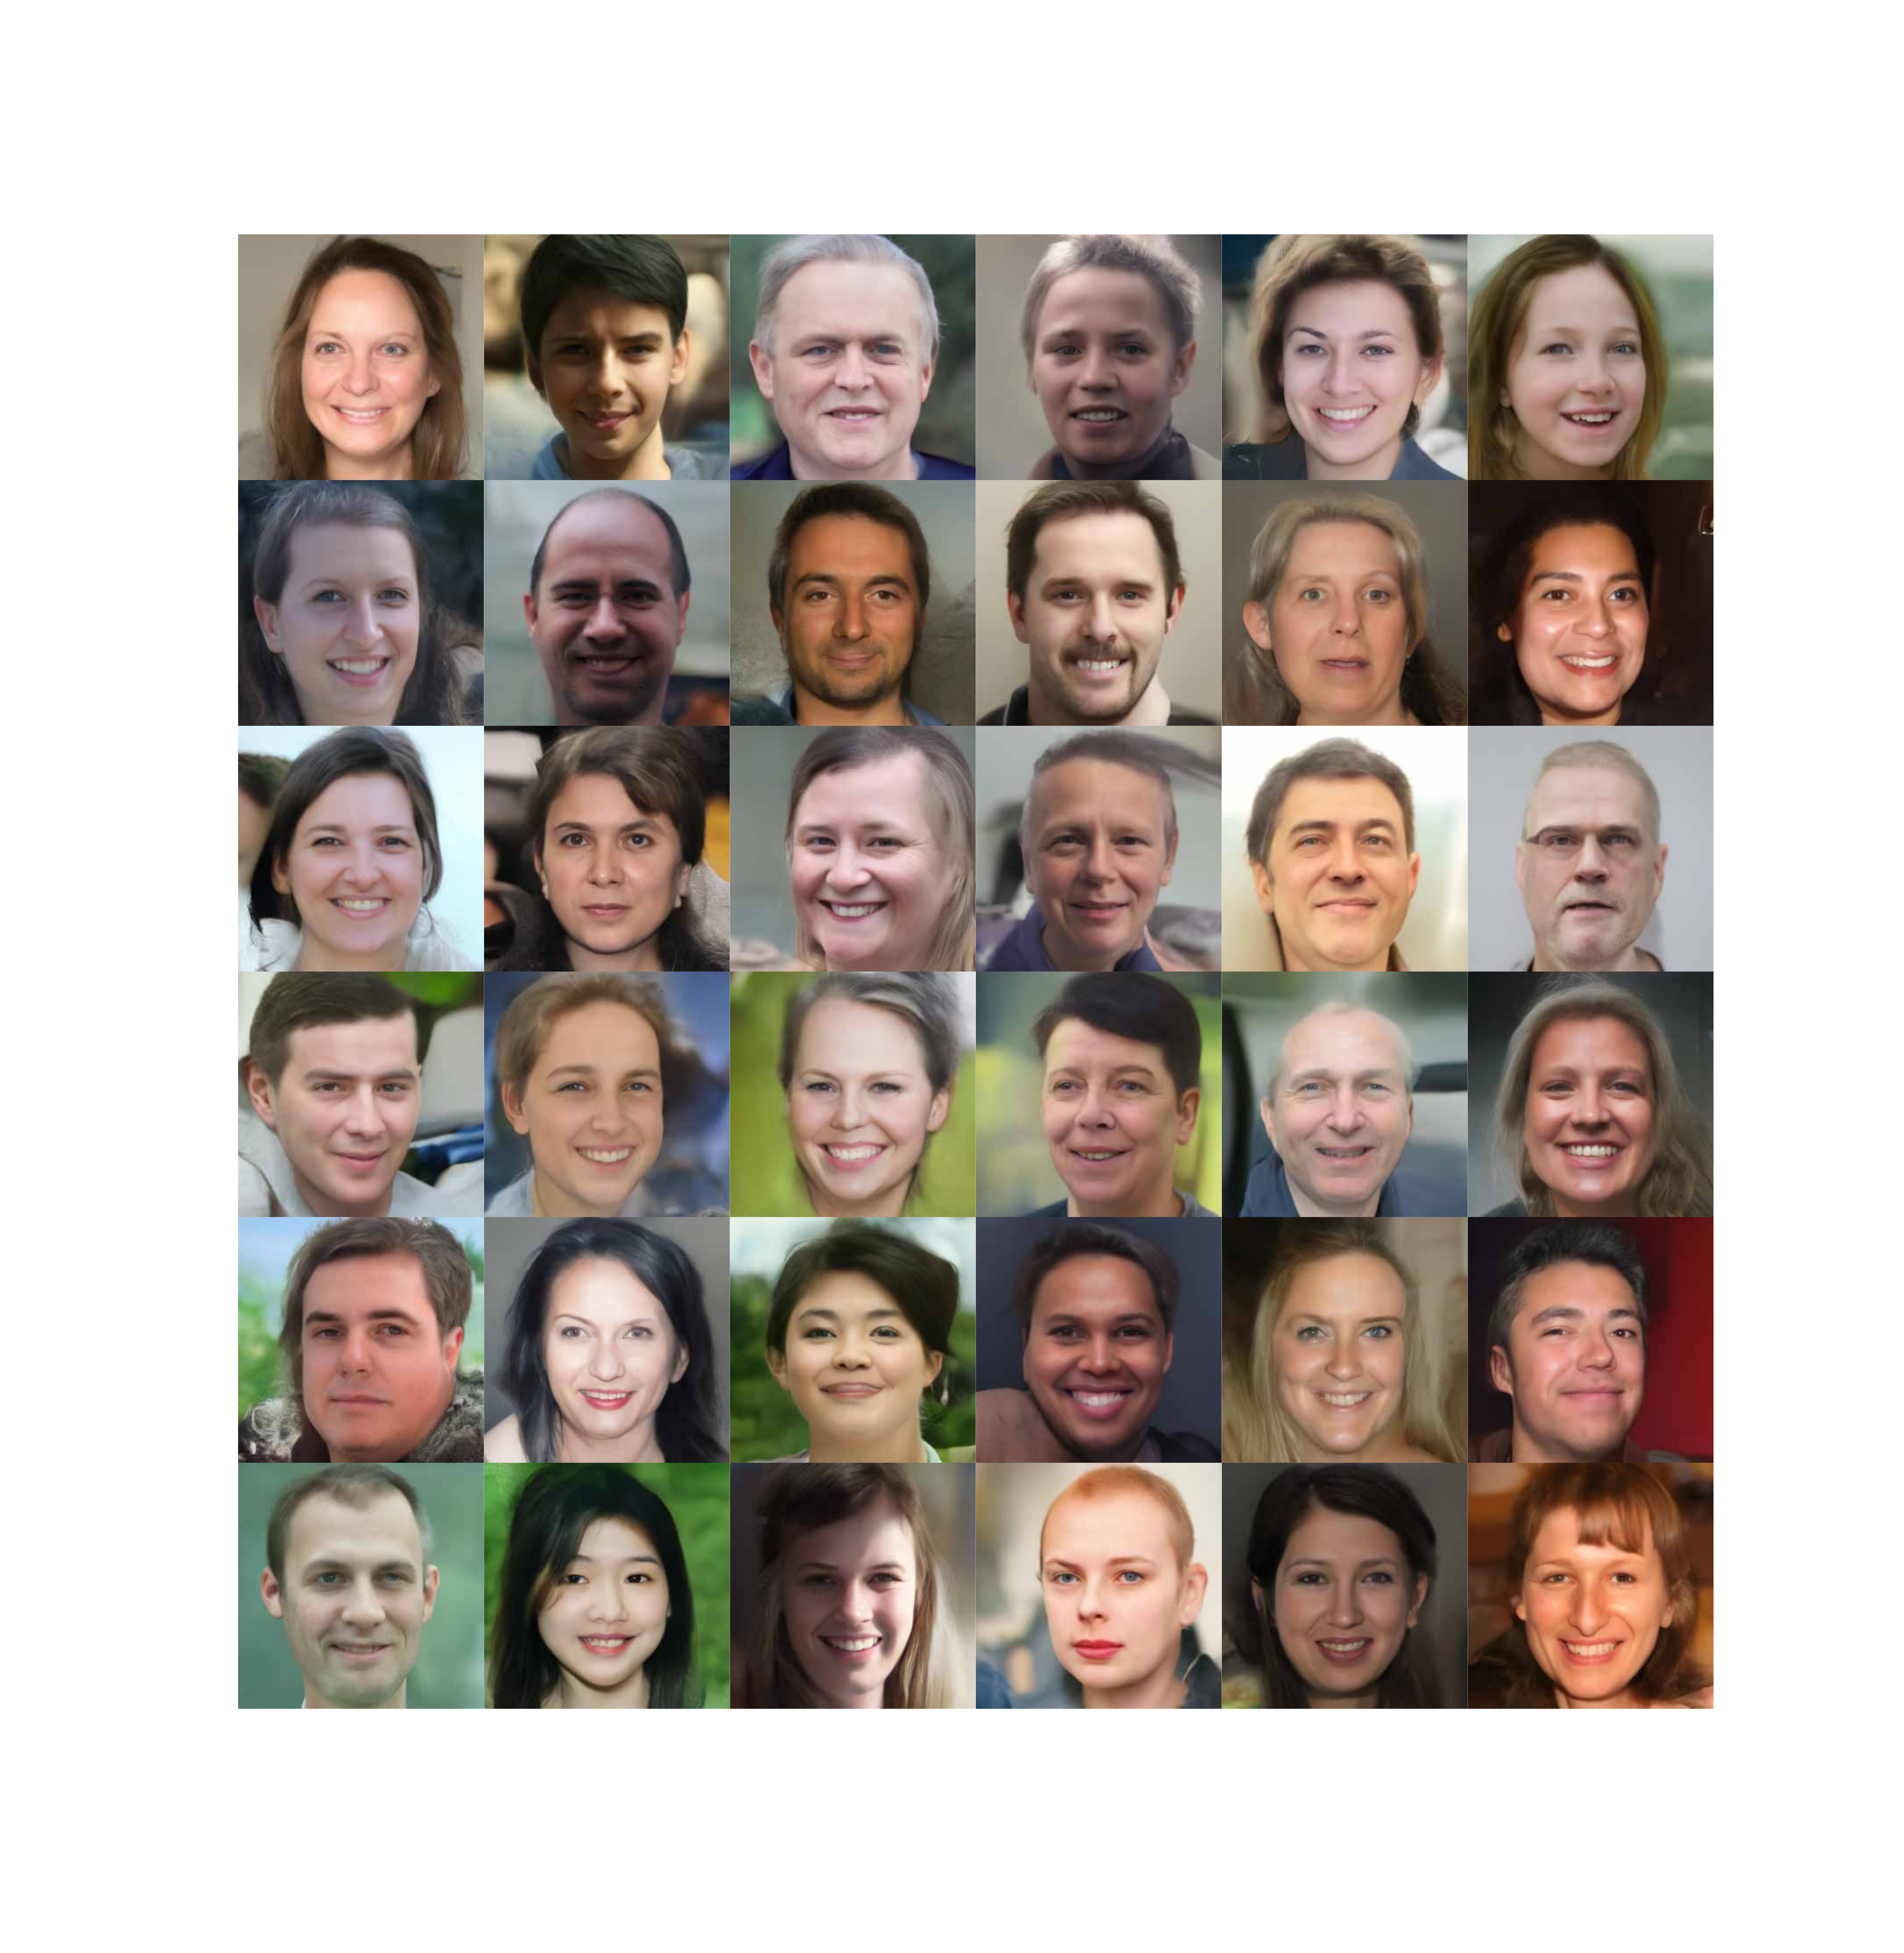}}
    \end{minipage}

    \vspace{-12ex}
        \caption{
        Facial images at a resolution of $1024\times 1024$ generated by NCSN++~\cite{song2020score}
        with our PDS using different solenoidal items.
        Sampling iterations: $66$.
        Dataset: FFHQ~\cite{karras2019style}.
    		}
        \label{fig:ffhq_s_ms}
        \vspace{-4ex}
\end{figure}
