# Supplementary material for: Accelerating Score-based Generative Models with Preconditioned Diffusion Sampling
Source: arXiv:2207.02196 source file (2022-12-05)
Supplement: Supplementary file 12 [file fid.tex]

\begin{table}[h]
\begin{center}
\caption{Quantitative evaluation with the Clean-FID (Fr\'echet Inception Distance) metric~\cite{parmaraliased} for accelerated diffusion process. We generate $50k$ images for each method.}\label{tab:fid}
\setlength{\tabcolsep}{2.3mm}{
\begin{tabular}{c|cc|ccc}
\toprule[1.5pt]
Model  & \multicolumn{2}{c|}{NCSNv2~\cite{DBLP:conf/nips/0011E20}}& \multicolumn{3}{c}{NCSN++~\cite{song2020score}} \\ \midrule
Dataset  & \multicolumn{1}{c}{LSUN} & \multicolumn{1}{c|}{LSUN} & \multicolumn{1}{c}{LSUN} & \multicolumn{1}{c}{LSUN} & \multicolumn{1}{c}{FFHQ} \\ \midrule
Class & \multicolumn{1}{c}{Church} & \multicolumn{1}{c|}{Tower} & \multicolumn{1}{c}{Bedroom} & \multicolumn{1}{c}{Church} & \multicolumn{1}{c}{Face} \\ \midrule
Resolution &
\multicolumn{1}{c}{$96\times96$} & \multicolumn{1}{c|}{$128\times128$} & \multicolumn{1}{c}{$256\times256$} & \multicolumn{1}{c}{$256\times256$} & \multicolumn{1}{c}{$1024\times1024$}
\\ \midrule
\multicolumn{1}{l|}{Iterations} & 156                                                                          & 108                                                                          & 166                                                                           & 166                                                                          & 66                                                                           \\
\midrule
Vanilla      & 217.9                                                                       & 67.2                                                                        & 393.7                                                                         & 393.3                                                                        & 463.2                                                                       \\
\textbf{PDS} & \textbf{65.7}                                                                & \textbf{43.8}                                                               & \textbf{16.9}                                                                 & \textbf{15.0}                                                                & \textbf{61.2}                                                                     \\ \bottomrule[1.5pt]
\end{tabular}}
\end{center}
\end{table}
